# Supplementary material for: Migration of gold atoms into a thiol-bonded molecular self-assembled monolayer, forming a cluster exhibiting a Coulomb staircase
Source: arXiv:2512.18931 source file (2025-12-22)
Supplement: Supplementary file 1 [file Coulomb_Staircase_Paper_SI_20251121.pdf]

# Supplementary information for: Migration of gold atoms into a thiol-bonded molecular self-assembled monolayer, forming a cluster exhibiting a Coulomb staircase

Bingxin Li<sup>1\*†</sup>, Shanglong Ning<sup>1\*†</sup>, Chunyang Miao<sup>1\*†</sup>, Chenyang Guo<sup>1</sup>,  
Gyu Don Kong<sup>3</sup>, Xintai Wang<sup>1</sup>, Victor I. Coldea<sup>1</sup>, Yuqiao Li<sup>1</sup>, Sam Harley<sup>2</sup>,  
Oleg V. Kolosov<sup>2</sup>, James Newson<sup>2</sup>, Sam Jarvis<sup>2</sup>, Ben Robinson<sup>2</sup>,  
Mohammed Alzanbaqi<sup>2</sup>, Ali Ismael<sup>2</sup>, Colin Lambert<sup>2</sup>, Hyo Jae Yoon<sup>3</sup>,  
Jeremy J. Baumberg<sup>1</sup>, Christopher J. B. Ford<sup>1\*</sup>

<sup>1\*</sup>Cavendish Laboratory, University of Cambridge, J J Thomson Avenue, Cambridge, CB3 0US, United Kingdom.

<sup>2</sup>Physics Department, Lancaster University, Lancaster, LA1 4YB, United Kingdom.

<sup>3</sup>Department of Chemistry, Korea University, Seoul, 02841, Korea.

\*Corresponding author(s). E-mail(s): [bl497@cantab.ac.uk](mailto:bl497@cantab.ac.uk); [sn538@cantab.ac.uk](mailto:sn538@cantab.ac.uk);  
[cm2109@cam.ac.uk](mailto:cm2109@cam.ac.uk); [cjbf@cam.ac.uk](mailto:cjbf@cam.ac.uk);

<sup>†</sup>These authors contributed equally to this work.

## 1 Theory of classical Coulomb blockade

In metallic quantum dots, where the energy levels form a continuum or are more closely spaced than the thermal energy  $k_B T$ , the energy spacing is negligible and the addition energy is just the charging energy  $E_{\text{add}} \approx \frac{e^2}{C_\Sigma}$ . By considering the average current flowing through barrier  $i$  (1, 2 for left or right) and using Fermi's Golden Rule, one can obtain the tunneling rate  $\gamma_i^\pm$  across barrier  $i$  as

$$\gamma_i^\pm(n) = \frac{1}{R_i e^2} \left[ \frac{-\Delta E_i^\pm}{1 - \exp(\Delta E_i^\pm / k_B T)} \right], \quad (\text{S1})$$

where  $\Delta E_i$  is the change in energy of the system when an electron tunnels across the barrier [1]. The tunneling resistance  $R_i \equiv h / (e^2 D_i D_d |T_i|^2)$ , and  $D_i$  and  $D_d$  represent the densities of states (assumed constant) for lead  $i$  and the metallic dot, respectively [2].  $T_i$  is the transmission probability of the barrier.

To account for the strongly varying density of states in graphene near the Dirac point—particularly its linear energy dependence—we introduce bias-dependent scaling parameters  $B$  and  $C$  that modify the effective energy change:  $\Delta E_{\text{eff}} = (1 + B)\Delta E$  for negative-bias regimes and  $\Delta E_{\text{eff}} = (1 + C)\Delta E$  for positive-bias regimes. These parameters quantitatively capture the asymmetric band-structure effects evident in our experimental data.

The current flowing through the two tunneling barriers is given by

$$I(V) = e \sum_{N=-\infty}^{\infty} \sigma(N) [\gamma_i^+ - \gamma_i^-], \quad (\text{S2})$$

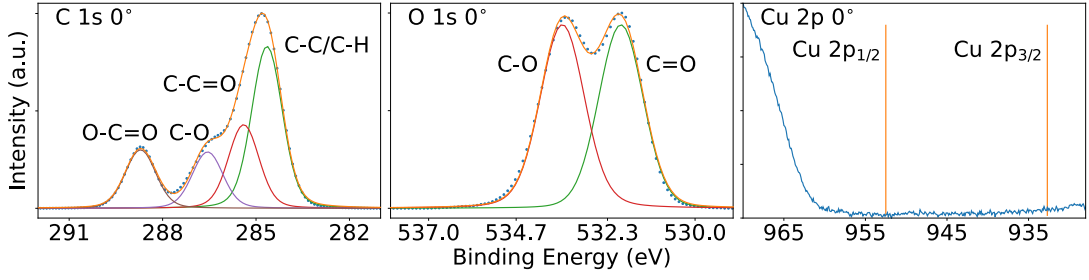

**Fig. S1:** Single-layer graphene on PMMA: XPS, with the X-ray beam at normal incidence, in the O 1s, C 1s, and Cu 2p regions of energy.

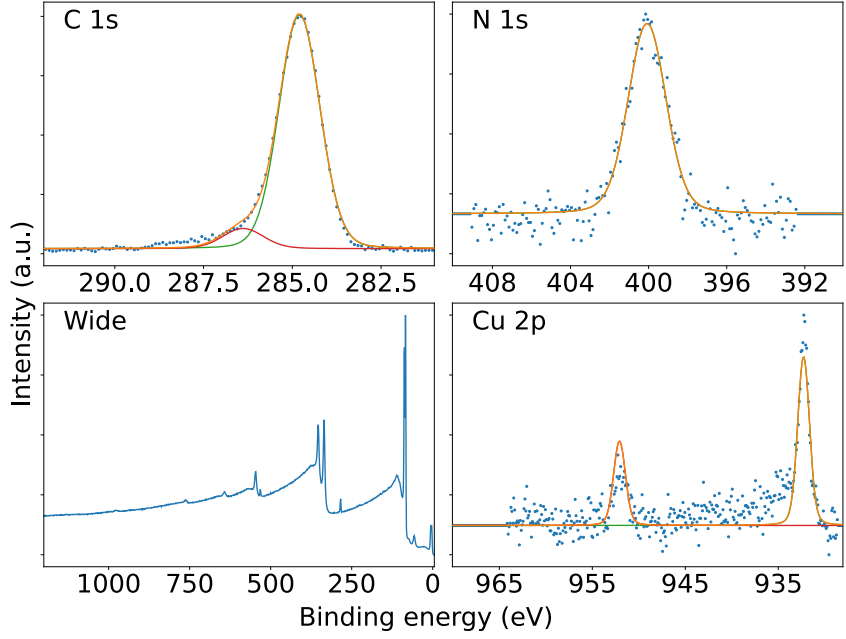

**Fig. S2:** XPS on a C16N SAM.

where  $\sigma(N)$  is the ensemble probability distribution of the number  $N$  of electrons on the dot, with  $\sum_{n=-\infty}^{\infty} \sigma(N) = 1$ . One can then solve simultaneously for each  $\sigma(N)$  from the steady-state case where the net probability of making a transition between two adjacent states  $N$  and  $N + 1$  is zero,

$$\sigma(N)[\gamma_1^+(N) + \gamma_2^+(N)] = \sigma(N + 1)[\gamma_1^-(N + 1) + \gamma_2^-(N + 1)], \quad (\text{S3})$$

by assuming that  $\sigma(N) = 0$  for values of  $|N| > 20$ , say.

## 2 XPS Measurements

As described in the main paper, Fig. S1 shows XPS in the O 1s, C 1s, and Cu 2p regions of energy, showing results typical of graphene on PMMA. Despite using exceptionally long acquisition times, and attempts to increase surface sensitivity using grazing-angle XPS, no Cu 2p was identified, indicating that the transfer process does not introduce any detectable Cu impurities from the Cu substrate on which the graphene was grown.

Similarly, Fig. S2 shows XPS on a C16N SAM. The single peak shows that the amine self-assembles well. There is a very weak Cu 2p signal, corresponding to an atomic percentage below 0.15%, which we attribute to solvent contamination. No other contamination signals were identified.

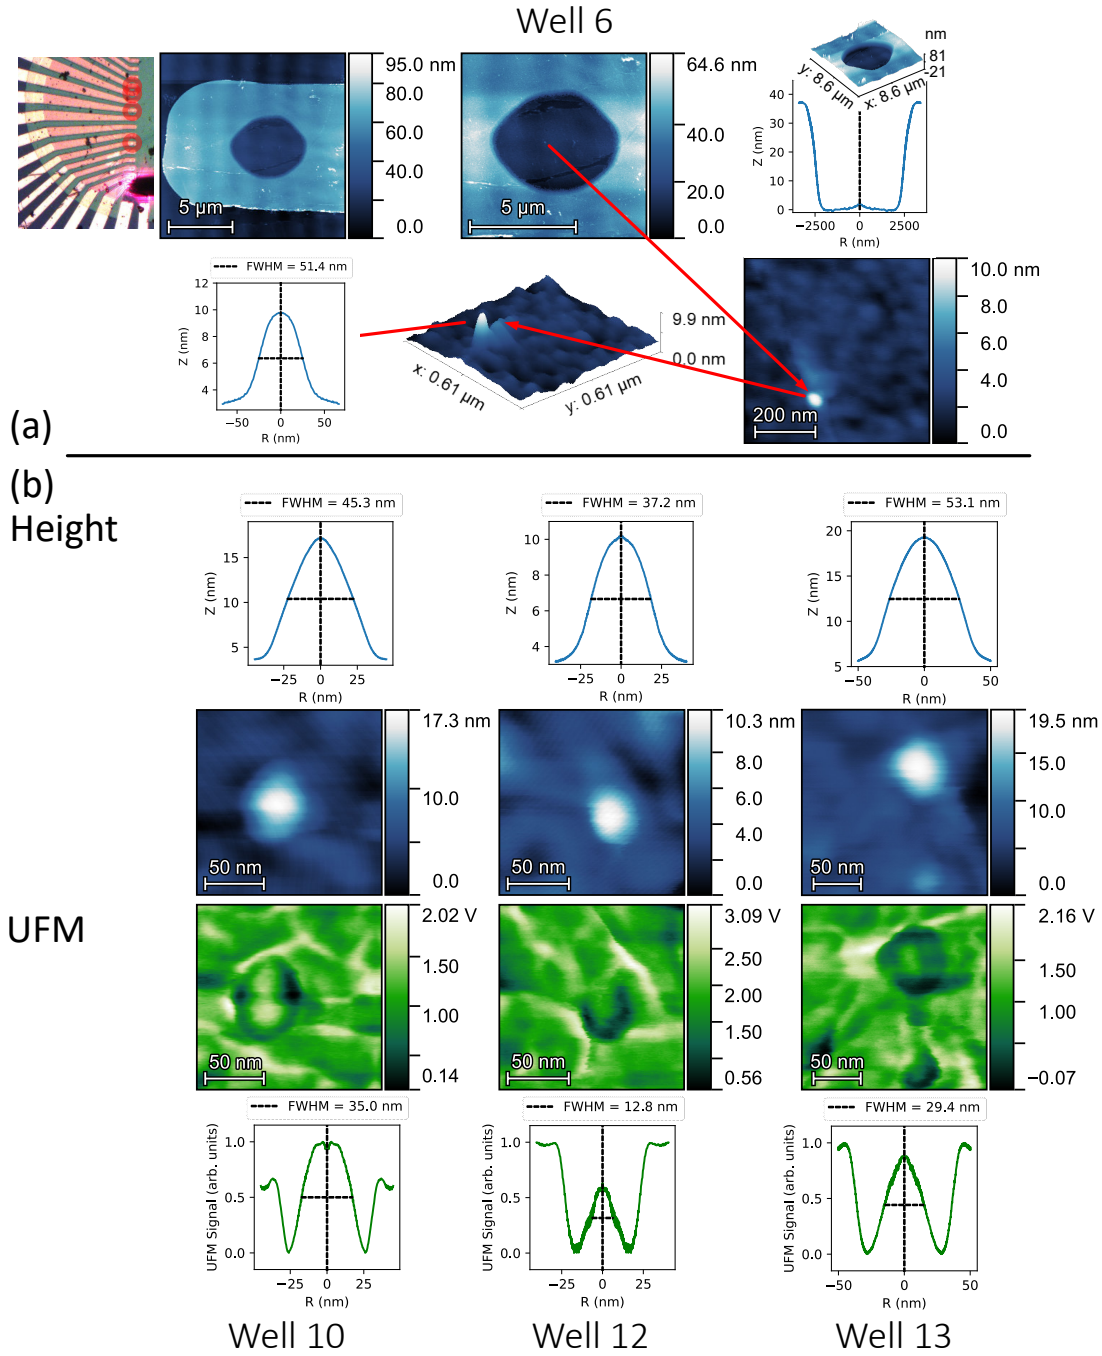

**Fig. S3:** (a) AFM on well 6, showing the whole well with a diameter of about 6  $\mu\text{m}$ . The well contains the usual Au-SAM-graphene sandwich, on top of which are some imperfections (white marks). The red arrows show that one of these was imaged at high resolution, to find a peak with FWHM  $\sim 50$  nm and height less than 10 nm. (b) AFM and UFM on bumps in wells 10, 12 and 13. The SAM employed is HSC11BIPY.

### 3 Force-microscopy results

Height maps of a series of microwell SAM devices on one chip that had already been measured were captured with a PeakForce tapping atomic force microscope (AFM). Radially averaged line profiles were extracted to show the wall shape. Small circular features were observed,  $< 100$  nm in diameter and  $< 10$  nm in height, see Fig. S3.

For most of these wells, ultrasonic force microscopy (UFM) was used to detect unsupported regions of graphene. High-resolution mapping of individual features from multiple wells shows that they are mostly unsupported, with a smaller supported region at the center. This suggests

that these features are caused by protrusions underneath the graphene. Wells 10–13 were examined by UFM. No features were found in well 11. The wells in Fig. S3(b) contain height and UFM images, as well as radially-averaged 1D line profiles (mirrored about the  $x$ -axis for ease of interpretation).

Topographical and nanomechanical mapping by AFM reveals the presence of small ( $< 40$  nm) features buried beneath the graphene. Extracting the true diameter of the buried feature from the UFM would require more analysis, and a better idea of the probe shape. The full-width half-maximum (FWHM) values calculated here are a reasonable upper bound on the diameter. These are somewhat larger than the diameters calculated from the capacitances from fitting the Coulomb staircase results. Interestingly, junction 11 showed a good staircase, but no detectable bump, whereas the other wells shown here showed less regular behavior, indicating perhaps that the clusters that are small enough to give good Coulomb blockade are smaller than those that are detectable even with the best AFM and UFM measurements. Also, the size may be slightly larger than in the electrical measurements, as about a year had passed since those were carried out.

## 4 Computational modeling of thiol-Au and amine-Au surface interactions

### 4.1 Optimized DFT Structures of Isolated Molecules

Using the density-functional code SIESTA[3, 4], the optimum geometries of the isolated molecules were obtained by relaxing the molecules until all forces on the atoms were less than  $0.01$  eV/Å, as shown in Fig. S4. A double-zeta plus polarization orbital basis set, norm-conserving pseudopotentials, with an energy cut-off of 250 Rydbergs, defined on the real-space grid was used and the local-density approximation (LDA) was chosen to be the exchange-correlation functional. We also computed results using GGA and found that the resulting functions were comparable with those obtained using LDA.[5, 6]

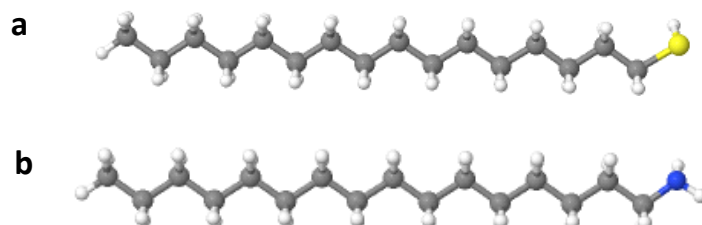

**Fig. S4:** Fully relaxed isolated alkane chain derivatives. a) 1-hexadecanethiol ( $\text{CH}_3(\text{CH}_2)_{15}\text{SH}$ , abbreviated to  $\text{C}_{16}\text{S}$ ) and b)  $\text{C}_{16}\text{N}$ .

### 4.2 Frontier orbitals of alkane chain derivatives

Figures S5 and S6 show isosurfaces of the HOMO, LUMO, HOMO–1 and LUMO+1 of isolated chain molecules (a)  $\text{C}_{16}\text{S}$  and (b)  $\text{C}_{16}\text{N}$  along with their energies.

### 4.3 Binding-energy simulations

The Au-amine and Au-thiol binding energies play a crucial role in determining the strength of molecule–surface interactions. The binding energy is crucial to the chemical stability of the junction as well as its electronic properties [7, 8]. Therefore, to begin the calculations, the optimum binding distance (corresponding to the optimum binding energy) between Au-amine and Au-thiol was simulated using DFT and the counterpoise method, which removes basis-set superposition errors (BSSE), as described in [7, 9–11]. In the case of Au-SH, it is known that the H is detached from the thiol group upon binding to gold and therefore the simulated junctions involve Au-S binding.

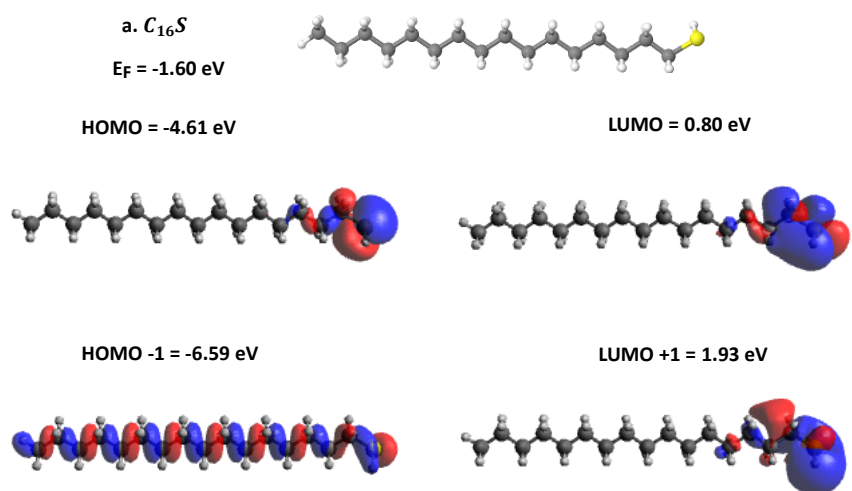

**Fig. S5:** The wave function of a  $C_{16}S$  molecule: Top panel: Fully optimized geometry. Lower panel: HOMO, LUMO, HOMO-1 and LUMO+1 along with their energies.

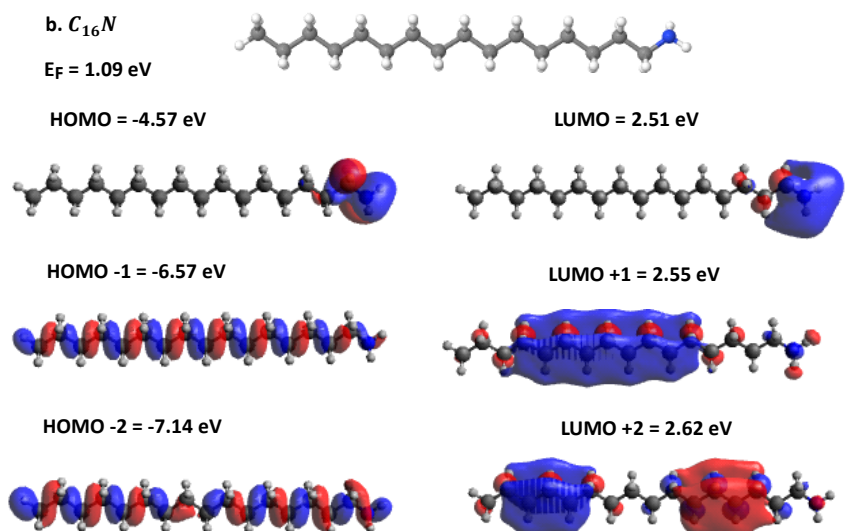

**Fig. S6:** The wave function of a  $C_{16}N$  molecule: Top panel: Fully optimized geometry. Lower panel: HOMO, LUMO, HOMO-1, LUMO+1, HOMO-2 and LUMO+2 along with their energies.

After optimizing the binding geometries of the chains to a gold substrate, the total energy as a function of the position of the gold atoms was calculated.

To balance computational accuracy with feasibility, a tiered approach to modeling the channels formed from clusters of molecular chains was employed: for the initial calculation, full-length single chains (specifically  $C_{16}S$  and  $C_{16}NH_2$ ) were used. This ensures an accurate description of all intramolecular interactions and electronic effects within an isolated molecule. To manage the significant computational cost associated with larger multi-chain systems (3 and 4 chains), the chain length was reduced by half (e.g., to  $C_8S$  and  $C_8NH_2$ ). This approximation is justified, as the core interactions governing assembly-head-group binding and inter-chain van-der-Waals forces are preserved. The terminal functional group, which is the focus of this energy-difference study, remains explicitly modeled. This strategy allows for an efficient yet representative investigation of the energetic landscape across different system sizes.

### 4.3.1 Single-chain simulations without a graphene top layer

The optimum lateral separation between a Au-1-chain and a Au atom was calculated, as indicated by the black arrow on the right panel of Figures S7 and S8 for both thiol and amine, respectively.

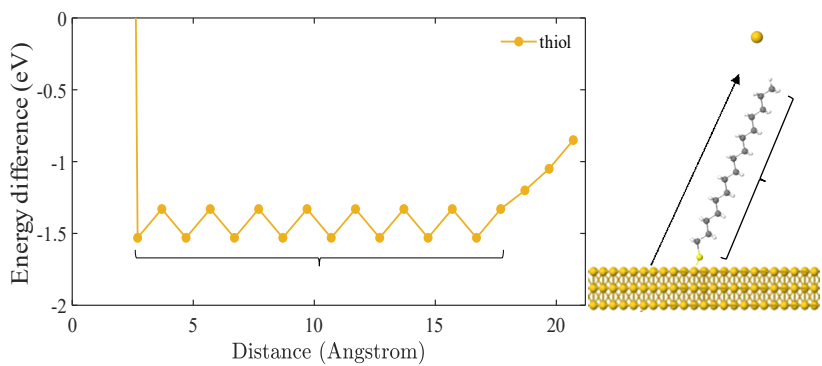

**Fig. S7:** Left panel: Binding energy as a function of the optimum binding distance  $d$  of thiol-anchored Au-1-chain and a Au atom. Right panel: Schematic representing a Au-1-chain and a Au atom moving along the 1-chain.

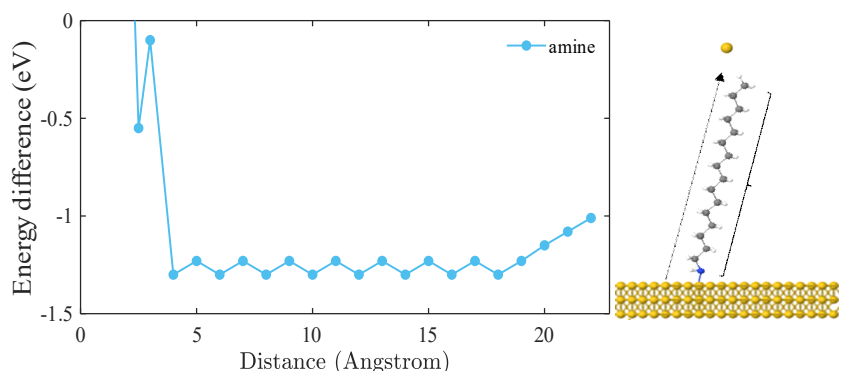

**Fig. S8:** As Fig. S7 for an amine-anchored Au-1-chain.

### 4.3.2 Multi-chain simulations without a graphene top layer

As noted previously, for multi-chain simulations the chain length was halved to reduce computational expense. Since the amine chain presents a large energy barrier that traps a Au atom, we focus on the thiol simulations. The optimum lateral separation between Au-multi-chains (3 and 4 chains), and a Au atom was calculated, as indicated by the black arrow on the right panel of Figs. S9 and S10, respectively. The chains were reduced to  $C_8S$  as shown in the Figures.

### 4.3.3 Multi-chain simulations with a graphene top layer

A graphene sheet was incorporated on top of the self-assembled monolayer to accurately simulate the conditions of experimental measurements. The optimum lateral separation between three Au chains and a Au atom, with graphene on top, was calculated as indicated by the black arrow on the right panel of Fig. S11. The chains are reduced to  $C_8S$  as shown in the Figure. The corresponding 4-chain simulations are shown in the main text (Fig. 4).

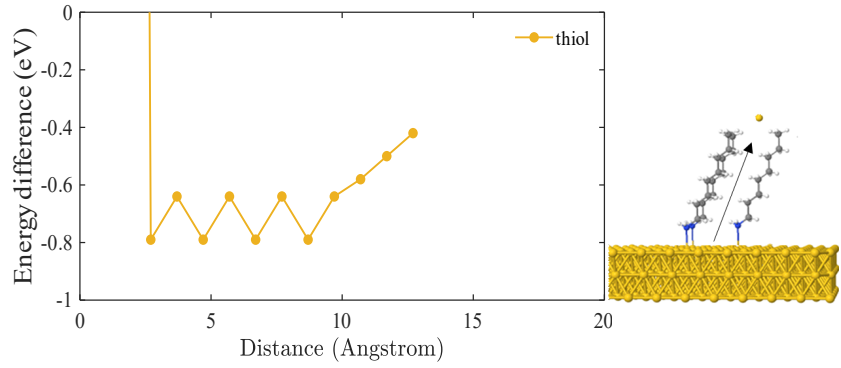

**Fig. S9:** As Fig. S7 for a thiol-anchored Au-3-chain.

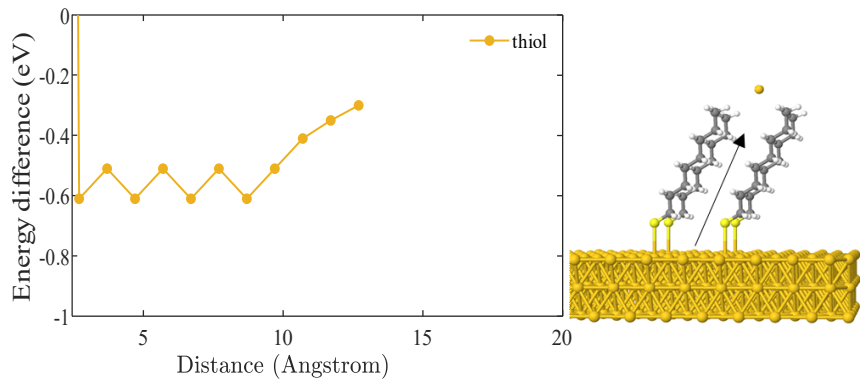

**Fig. S10:** As Fig. S7 for a thiol-anchored Au-4-chain.

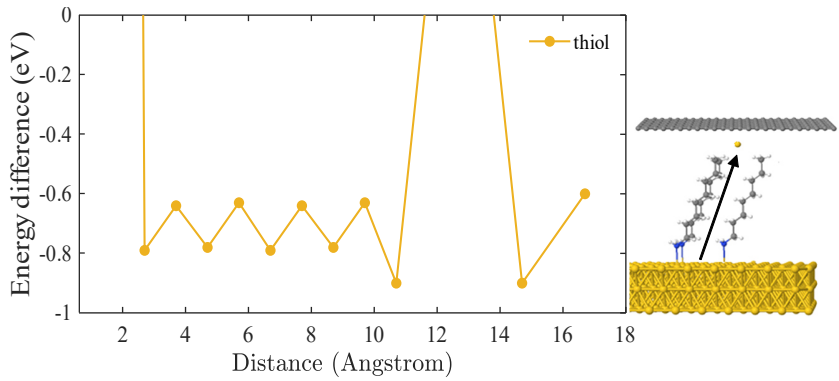

**Fig. S11:** As Fig. S7 for a thiol-anchored Au-3-chain with graphene on top.

## References

- [1] Hanna, A.E., Tinkham, M.: Variation of the Coulomb staircase in a two-junction system by fractional electron charge. *Phys. Rev. B* **44**(11), 5919–5922 <https://doi.org/10.1103/PhysRevB.44.5919>
- [2] Amman, M., Wilkins, R., Ben-Jacob, E., Maker, P.D., Jaklevic, R.C.: Analytic solution for the current-voltage characteristic of two mesoscopic tunnel junctions coupled in series. *Phys. Rev. B* **43**(1), 1146–1149 <https://doi.org/10.1103/PhysRevB.43.1146>
- [3] Soler, J.M., Artacho, E., Gale, J.D., García, A., Junquera, J., Ordejón, P., Sánchez-Portal, D.: The SIESTA method for ab initio order-N materials simulation. *J. Phys.: Condens. Matter* **14**(11), 2745 (2002) <https://doi.org/10.1088/0953-8984/14/11/302>
- [4] Artacho, E., Anglada, E., Diéguez, O., Gale, J.D., García, A., Junquera, J., Martín, R.M., Ordejón, P., Pruneda, J.M., Sánchez-Portal, D., Soler, J.M.: The SIESTA method; developments and applicability. *J Phys*

Condens Matter **20**(6), 064208 (2008) <https://doi.org/10.1088/0953-8984/20/6/064208>

- [5] Ismael, A.K., Lambert, C.J.: Single-molecule conductance oscillations in alkane rings. *J. Mater. Chem. C* **7**(22), 6578–6581 (2019) <https://doi.org/10.1039/C8TC05565C>
- [6] Gantenbein, M., Wang, L., Al-Jobory, A.A., Ismael, A.K., Lambert, C.J., Hong, W., Bryce, M.R.: Quantum interference and heteroaromaticity of para- and meta-linked bridged biphenyl units in single molecular conductance measurements. *Sci. Rep.* **7**(1), 1794 (2017) <https://doi.org/10.1038/s41598-017-01903-0>
- [7] Obersteiner, V., Egger, D.A., Zojer, E.: Impact of Anchoring Groups on Ballistic Transport: Single Molecule vs Monolayer Junctions. *J. Phys. Chem. C* **119**(36), 21198–21208 (2015) <https://doi.org/10.1021/acs.jpcc.5b06110>
- [8] Lukas, M., Dössel, K., Schramm, A., Fuhr, O., Stroh, C., Mayor, M., Fink, K., Löhneysen, H.: A tripodal molecule on a gold surface: orientation-dependent coupling and electronic properties of the molecular legs. *ACS Nano* **7**(7), 6170–6180 (2013) <https://doi.org/10.1021/nn4020505>
- [9] Herrer, L., Ismael, A., Martín, S., Milan, D.C., Serrano, J.L., Nichols, R.J., Lambert, C., Cea, P.: Single molecule vs. large area design of molecular electronic devices incorporating an efficient 2-aminepyridine double anchoring group. *Nanoscale* **11**(34), 15871–15880 (2019) <https://doi.org/10.1039/C9NR05662A>
- [10] Kobko, N., Dannenberg, J.: Effect of Basis Set Superposition Error (BSSE) upon ab Initio Calculations of Organic Transition States. *J. Phys. Chem. A* **105**, 1944–1950 (2001) <https://doi.org/10.1021/jp001970b>
- [11] Sherrill, C.D.: Counterpoise correction and basis set superposition error. <https://vergil.chemistry.gatech.edu/notes/cp.pdf> (2010)
